# Supplementary material for: Dynamic mass generation on two-dimensional electronic hyperbolic lattices
Source: arXiv:2302.04864 ancillary file (2025-03-21)
Supplement: Supplementary file 1 [file Supplementary.pdf]

# Supplementary Material: Dynamic mass generation on two-dimensional electronic hyperbolic lattices

Noble Gluscevich,[1,*] Abhisek Samanta,[2,*] Sourav Manna,[3,4] and Bitan Roy[1,†]

[1]Department of Physics, Lehigh University, Bethlehem, Pennsylvania, 18015, USA
[2]Department of Physics, The Ohio State University, Columbus, Ohio 43210, USA
[3]Department of Condensed Matter Physics, Weizmann Institute of Science, Rehovot 7610001, Israel
[4]Raymond and Beverly Sackler School of Physics and Astronomy, Tel-Aviv University, Tel Aviv 6997801, Israel

(Dated: February 9, 2023)

The Supplementary Material contains (a) solutions of the self-consistent gap equation for dynamic mass generation in Dirac and Fermi liquids [Sec. S1] and (b) additional numerical results on the self-consistent solutions of the charge-density-wave (CDW) and antiferromagnet (AFM) orders on hyperbolic lattices, different from the ones shown in the main manuscript [Sec. S2, Figs. S1 and S2].

## S1. SELF-CONSISTENT GAP EQUATION AND ITS SOLUTIONS

The self-consistent mean-field gap equation, capturing dynamic mass ($\Delta$) generation due to a local four-fermion interaction ($g$) takes the form [1, 2]

$$g \int_0^{E_\Lambda} dE \, \frac{\rho(E)}{[E^2 + \Delta^2]^{1/2}} = 1. \tag{S1}$$

Here the integration is performed over energy $E$, and $E_\Lambda$ is an ultraviolet energy cut-off up to which the density of states (DOS) $\rho(E)$ follows a particular functional dependence on $E$. Here we analytically solve this equation for (i) Dirac liquids with $\rho(E) = \rho_0 |E|$ and (ii) Fermi liquids with $\rho(E) = \rho_0$, where $\rho_0$ is a constant.

In Dirac liquids, the integral on the left hand side of the gap equation is ultraviolet (UV) divergent, yielding

$$\sqrt{\Delta^2 + E_\Lambda^2} - \Delta = \frac{1}{\rho_0 g}. \tag{S2}$$

The UV divergence can be regularized by introducing the critical coupling for the ordering as $g_c = (\rho_0 E_\Lambda)^{-1}$, obtained by setting $\Delta = 0$ on the left hand side of the above equation. To proceed further, we define the following dimensionless quantities $\delta = \Delta / E_\Lambda$, $\lambda = g \rho_0 E_\Lambda$ and $\lambda_c = g_c \rho_0 E_\Lambda$. The UV regularized solution of the gap equation then reads

$$\lambda - \lambda_c = \frac{1}{[1+\delta^2]^{1/2} - \delta} - 1. \tag{S3}$$

Notice that the right hand side is positive definite for $\delta > 0$. Therefore, nontrivial solution for dynamic mass generation in Dirac liquids can only be found when the interaction strength ($\lambda$) is above a critical interaction strength ($\lambda_c$), namely for $\lambda > \lambda_c$. Expanding the right hand side in powers of $\delta$, we obtain

$$\lambda - \lambda_c = \delta + \frac{\delta^2}{2} + \mathcal{O}(\delta^4). \tag{S4}$$

When $\lambda$ is very close to $\lambda_c$, $\delta \sim (\lambda - \lambda_c)$. But in this regime the lattice based numerical self-consistent solutions for any order parameter suffers from finite size effects. Thus, to pin $\lambda_c$, we move slightly away from this regime, such that the quadratic term dominates over the linear one, yielding $\delta \sim \sqrt{\lambda - \lambda_c}$. In this regime, the interaction strength dominates and the wavefunctions become more localized (Wannier-like), thus minimizing the finite size effects.

---

* Equal contributors

† Corresponding author: bitan.roy@lehigh.edu

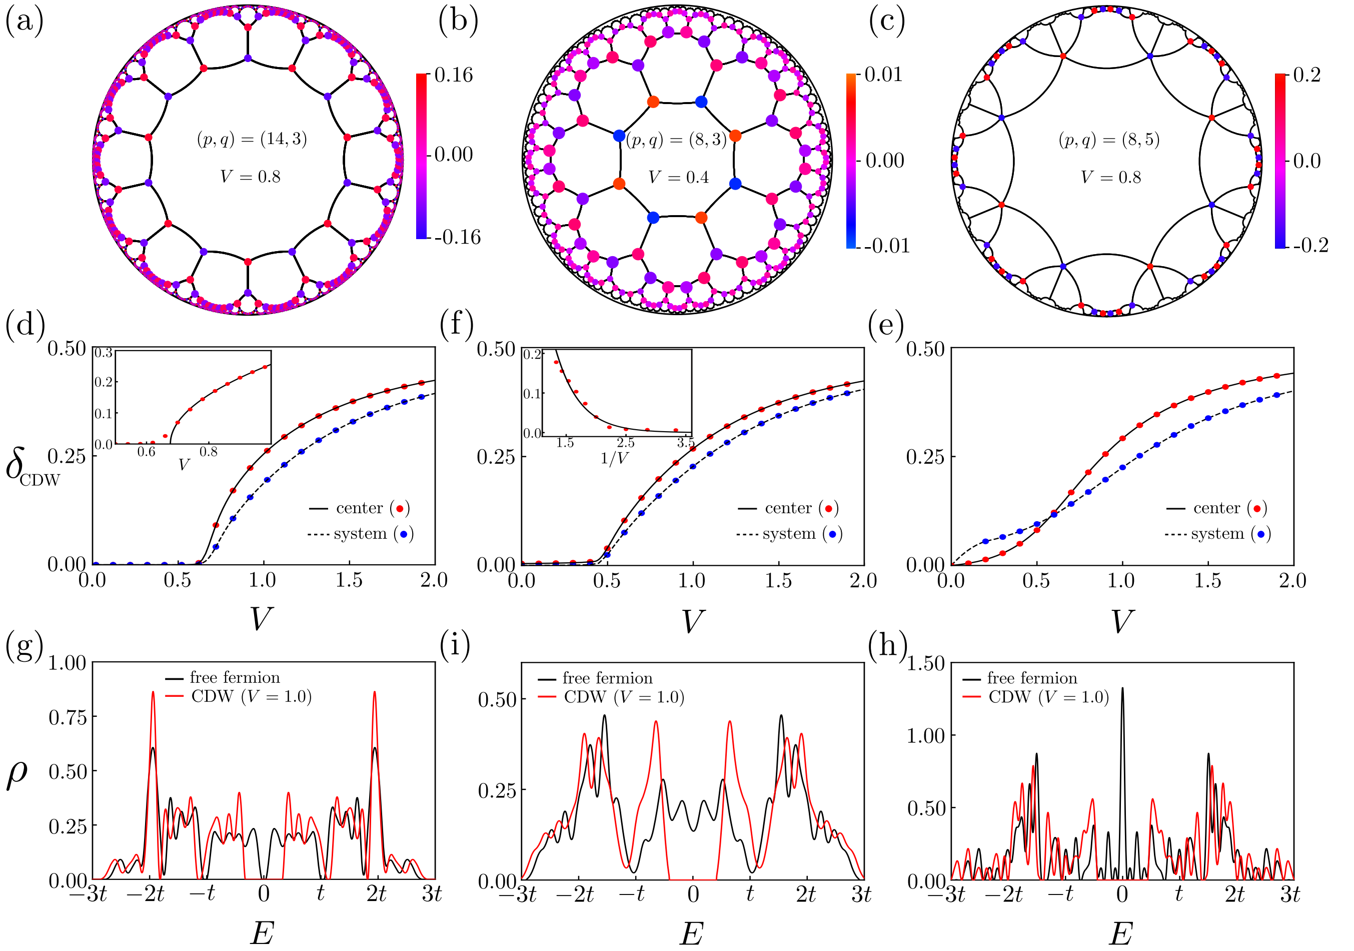


Figure S1. CDW ordering on hyperbolic lattices resulting from the NN Coulomb repulsion ($V$). The spatial variation of the average electronic density measured from the half-filling on (a) $(14,3)$, (b) $(8,3)$, and (c) $(8,5)$ hyperbolic lattices for $V=0.8$, 0.4 and 0.8, respectively. Scaling of the CDW order parameter with $V$ at the center (red) and averaged over the entire system (blue) in these systems are respectively shown in (d), (e), and (f). DOS for free fermions (black) and in the presence of the CDW order (red) in these systems are shown in (g), (h) and (i), respectively, for $V=1.0$, displaying the formation of an insulator at half-filling. Here, the results are presented for second generation $(14,3)$, fourth generation $(8,3)$ and second generation $(8,5)$ hyperbolic lattices, respectively containing 1694, 2888, and 384 sites. Critical coupling for the CDW ordering in $(14,3)$ Dirac system is estimated to be $V_c \approx 0.68$ [inset of (d)], while in $(8,3)$ Fermi liquids it follows the BCS scaling [inset of (e)].

The CDW and AFM orders are respectively denoted by $\delta_{\rm CDW}$ and $\delta_{\rm AFM}$. The corresponding interaction strengths are the nearest-neighbor Coulomb ($V$) and on-site Hubbard ($U$) repulsions, respectively. All these quantities are measured in units of the uniform NN hopping amplitude $t$ (set to be unity for the sake of convenience), and are thus dimensionless. We use the above scaling forms, namely $\delta_{\rm CDW} \sim \sqrt{V-V_c}$ and $\delta_{\rm AFM} \sim \sqrt{U-U_c}$ to determine $V_c$ and $U_c$, respectively, from lattice based numerical Hartree-Fock analyses. Here $V_c$ ($U_c$) is the critical NN Coulomb (on-site Hubbard) repulsion for the CDW (AFM) order.

In Fermi liquids the gap equation in Eq. (S1) after the integral over energy reads

$$g\rho_0 \ln\left(\frac{E_\Lambda + \sqrt{\Delta^2 + E_\Lambda^2}}{\Delta}\right) = 1. \tag{S5}$$

Restricting ourselves within the weak coupling regime, such that $\Delta \ll E_\Lambda$ or $\delta \ll 1$, we find the BCS scaling form of the mass ($\delta$) with the interaction strength ($g$)

$$\ln(\delta) = -\frac{1}{g\rho_0} \;\; \Rightarrow \;\; \delta = \exp\left(-\frac{\kappa}{g}\right), \tag{S6}$$

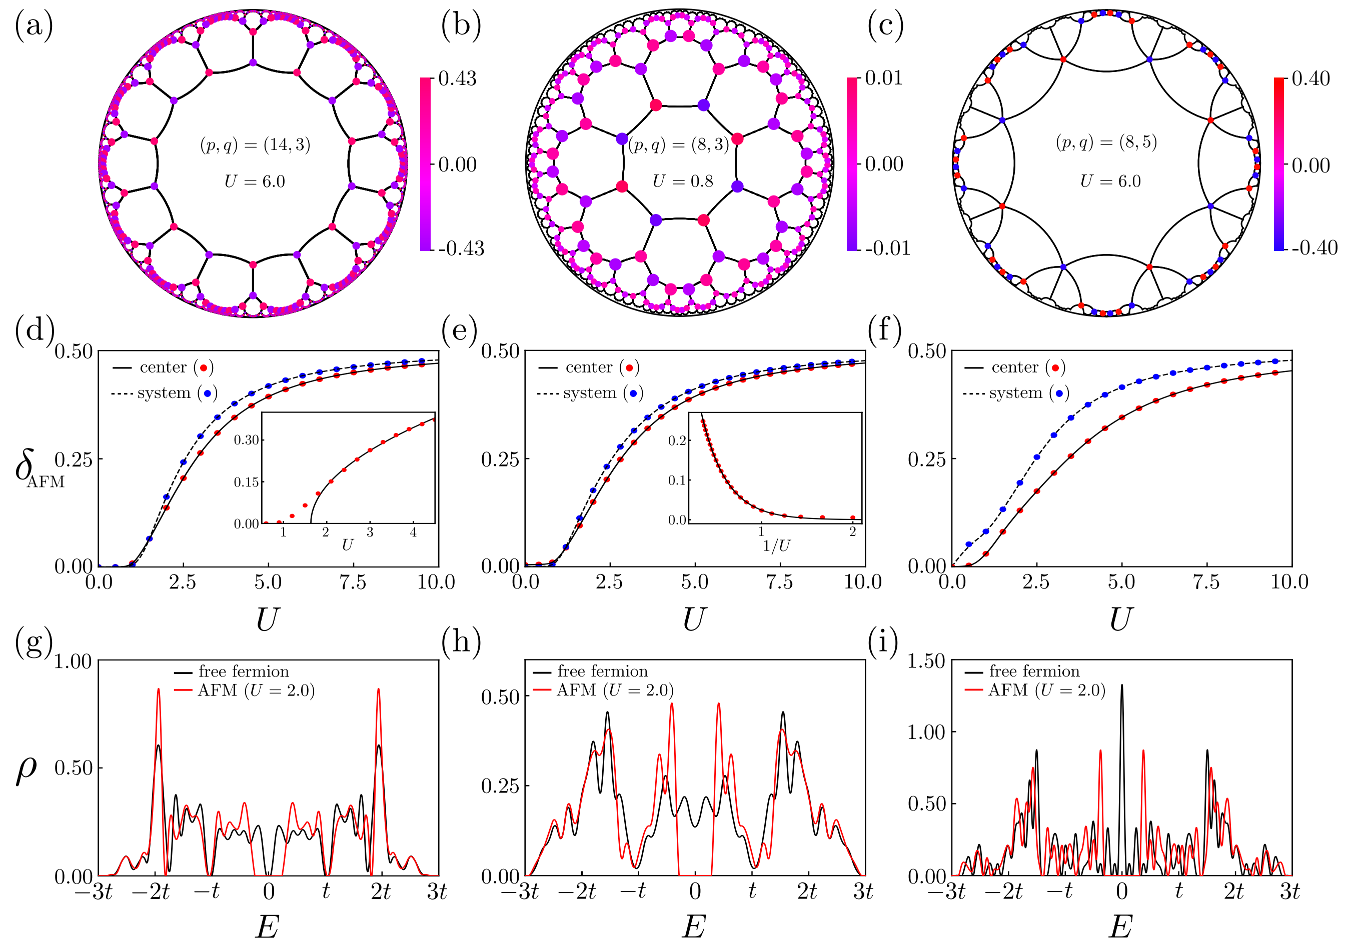


Figure S2. On-site Hubbard repulsion ($U$) mediated AFM ordering on hyperbolic lattices. All the details are the same as in Fig. S1, but for the AFM order (see main manuscript). Top row: Self-consistent solutions of magnetization at each site measured from its value at half-filling (zero), featuring the AFM order for $U = 6.0$, 0.8 and 6.0 respectively on $(14, 3)$, $(8, 3)$ and $(8, 5)$ hyperbolic lattices. Here, the results are presented for the same generation hyperbolic lattices as for the CDW ordering, mentioned in the caption of Fig. S1.

where $\kappa \equiv \rho_0^{-1}$ is a nonuniversal constant. Our numerical self-consistent solutions for the CDW and AFM orders respectively for weak NN Coulomb and on-site Hubbard repulsions on hyperbolic lattices supporting finite DOS at zero energy conform to this scaling form, where we treat $\kappa$ as a fitting parameter.

## S2. ADDITIONAL NUMERICAL RESULTS

In the main manuscript, we present lattice based self-consistent solutions for the CDW and AFM orders with NN and on-site repulsions, respectively. We presented these results on hyperbolic lattices featuring Dirac liquids, Fermi liquids, and flat bands around half-filling, characterized by vanishing, constant, and divergent DOS near the zero energy $\rho(0)$, respectively. As a prototypical representatives of these three classes of electronic fluids we focused on the $(10, 3)$, $(12, 3)$ and $(12, 4)$ hyperbolic lattices, respectively. However, as claimed in the main manuscript the respective scaling of the dynamically generated masses (such as CDW and AFM) is universal and it does not dependent on the corresponding choices of $(p, q)$, and only depend on the scaling of $\rho(E)$ around zero energy.

To anchor this claim, here we display the self-consistent solutions for the CDW and AFM orders in Fig. S1 and Fig. S2, respectively, on $(14, 3)$, $(8, 3)$ and $(8, 5)$ hyperbolic lattices. They accommodate hyperbolic Dirac liquid,

Fermi liquid, and flat band, respectively. See Table I of the main manuscript. For example, on $(14, 3)$ hyperbolic lattice $V_c = 0.68$ and $U_c = 1.62$, and on $(8, 3)$ hyperbolic lattice $\kappa = 2.49$ and $3.64$ for the CDW and AFM orders, respectively.

[1] B. Roy, Interacting nodal-line semimetal: Proximity effect and spontaneous symmetry breaking, Phys. Rev. B **96**, 041113 (2017).
[2] M. Tinkham, Introduction to Superconductivity (Dover Publication, New York, 2004).
